# Supplementary material for: Enhancing Security Control Production With Generative AI
Source: arXiv:2411.04284 source file (2024-11-06)
Supplement: Supplementary file 1 [file appendix.tex]

\section{Appendix}

\subsection{Detailed Description of Control Types}

\begin{enumerate}
\item \textbf{Encryption of data at rest} - Data at rest refers to data that's stored in persistent, non-volatile storage for any duration. Encrypting data at rest helps you protect its confidentiality, which reduces the risk that an unauthorized user can access it. This control detects where {resource} is encrypted at rest. If the resource {resource} is not encrypted at rest the control will return NON\_COMPLIANT. If the {resource} is encrypted it will return {COMPLIANT}

\item \textbf{Encryption of data in transit} - Data in transit refers to data that moves from one location to another, such as between nodes in your cluster or between your cluster and your application. Data may move across the internet or within a private network. Encrypting data in transit reduces the risk that an unauthorized user can eavesdrop on network traffic.

\item \textbf{Tagging} - A tag is a label that you assign to an AWS resource, and it consists of a key and an optional value. You can create tags to categorize resources by purpose, owner, environment, or other criteria. Tags can help you identify, organize, search for, and filter resources. Tagging also helps you track accountable resource owners for actions and notifications. When you use tagging, you can implement attribute-based access control (ABAC) as an authorization strategy, which defines permissions based on tags. You can attach tags to IAM entities (users or roles) and to AWS resources. You can create a single ABAC policy or a separate set of policies for your IAM principals. You can design these ABAC policies to allow operations when the principal's tag matches the resource tag.

\item \textbf{Resources run on supported version} - Running resources on supported software versions ensures optimal performance, security, and access to the latest features. Regular updates safeguard against vulnerabilities, guaranteeing a stable and efficient user experience.

\item \textbf{Backup enabled} - A data backup is a copy of your system, configuration, or application data that’s stored separately from the original. Enabling regular backups helps you safeguard valuable data against unforeseen events like system failures, cyberattacks, or accidental deletions. Having a robust backup strategy also facilitates quicker recovery, business continuity, and peace of mind in the face of potential data loss.

\item \textbf{Multi AZ} - An AZ is a distinct location within an AWS Region that is insulated from failures in other AZs. Enabling multiple AZs is recommended for enhanced resilience and fault tolerance in the event of infrastructure issues. Multi-AZ architectures aim to minimize the impact of infrastructure failures by dispersing resources across multiple AZs.

\item \textbf{Can inbound IP connections made to the resource} - Inbound connections can pose security risks by allowing unauthorized access to a system, leading to data breaches, system compromise, or exploitation of vulnerabilities. Robust security measures such as firewalls, access controls, and encryption are required to mitigate these risks.

\item \textbf{Can resource be accessed by anyone} - Publicly accessible resources can be lead to unauthorized access, data breaches or exploitation of vulnerabilities. Restricting access through authentication and authorization measures helps to safeguard sensitive information and maintain the integrity of your resources.

\item \textbf{Audit Logging enabled with destination log} - Audit logs track and monitor system activities. They provide a record of events that can help you detect security breaches, investigate incidents, and comply with regulations. Audit logs also enhance the overall accountability and transparency of your organization.
\end{enumerate}

\subsection{Evaluation Criteria}
The evaluation rubric is divided into two main categories: Scenario Evaluation (S) and Rule Evaluation (R). Each category contains specific criteria that the human evaluator must consider.

\subsubsection{Scenario Evaluation (S)}
\begin{enumerate}[leftmargin=*]
\item \textit{(S1) The number of scenarios recorded is correct}. This criterion assesses whether the generated Gherkin includes the appropriate number of scenarios. Each scenario should represent a distinct and necessary test case for the security control.
\item \textit{(S2) The field specified in the scenario exists}. This checks if all fields referenced in the scenarios are valid and present in the context of the security control being defined. It ensures the relevance and applicability of the scenarios.
\item \textit{(S3) The resulting compliance status is possible}. This criterion evaluates whether the compliance status derived from the scenario is feasible. It ensures that the scenarios result in legitimate compliance outcomes.
\item \textit{(S4) The configuration of the resource specified by the scenario is possible}. This ensures that the configuration actions described in the scenarios can actually be implemented within the given cloud environment. It checks for the practicality of the scenarios.
\item \textit{(S5) The conclusion of the scenario is correct}. This criterion checks if the scenario logically concludes with the correct outcome based on the preceding steps. It verifies the logical flow and correctness of the scenario's outcome.
\end{enumerate}

\subsubsection{Rule Evaluation (R)}
\begin{enumerate}[leftmargin=*]
\item  (R1) The rule name correctly describes the control specified by the collection of scenarios: This assesses the accuracy and appropriateness of the rule name. The rule name should succinctly and accurately reflect the control described by the scenarios.
\item (R2) The description correctly describes the control specified by the collection of scenarios: This criterion evaluates the clarity and correctness of the rule description, and whether it provides a clear understanding of the control and its purpose.
\end{enumerate}

\subsection{Scoring Mechanism}
The overall score for a Gherkin script is calculated using the following formula:
\begin{equation}
    score = (S1+S2+S3+S4+S5)\times (R1+R2)/2
\end{equation}
This formula integrates the evaluations from both the scenario and rule criteria, ensuring a comprehensive assessment of the Gherkin script's quality.
